# Supplementary material for: CAGS: Open-Vocabulary 3D Scene Understanding with Context-Aware Gaussian Splatting
Source: arXiv:2504.11893 source file (2025-04-16)
Supplement: Supplementary file 1 [file appendix.tex]

\section*{A Appendix}
\subsection*{A.1 Implementation Details}
\begin{enumerate}
    \item \textbf{Training Strategy:} In line with LangSplat, we commence by pre-training the standard 3DGS for 30,000 steps. Subsequently, we freeze the Gaussian coordinates, scale, and opacity parameters. Then, we train the instance features for 10,000 steps (for ScanNet, it is 20,000 steps) and the two-layer codebook for 30,000 steps (for ScanNet, it amounts to 40,000 steps). The 2D-3D feature association step does not require any training. The extraction methods for SAM masks and CLIP features are also in accordance with those of LangSplat. While LangSplat extracts three layers of SAM masks (small, middle, and large), our implementation utilizes only one layer, which is the large layer.
    \item \textbf{Training Time:} We carry out the training of each scene on a single 32G V100 GPU (with the actual memory usage fluctuating between approximately 16 to 20G). For the LERF dataset, each scene involves around 200 images and the training duration is roughly 50 minutes. For the ScanNet dataset, each scene consists of about 100-300 images (sampling every 20 frames from the original data and performing a downsampling by a factor of 2), and the training time is approximately 15 minutes. The 2D-3D feature association step is a one-time computation, and no additional computation is required during the inference phase. The association process takes around 1 minute.
    \item \textbf{ScanNet Dataset Evaluation:} We randomly selected 10 scenes from ScanNet for the evaluation purpose. These scenes are specifically: scene0000\_00, scene0062\_00, scene0070\_00, scene0097\_00, scene0140\_00, scene0200\_00, scene0347\_00, scene0400\_00, scene0590\_00, scene0645\_00. 
    The 19 categories (as defined by ScanNet) employed for text query are, respectively: wall, floor, cabinet, bed, chair, sofa, table, door, window, bookshelf, picture, counter, desk, curtain, refrigerator, shower curtain, toilet, sink, bathtub. Among them, 15 categories exclude picture, refrigerator, shower curtain, and bathtub. Moreover, 10 categories further exclude cabinet, counter, desk, curtain, and sink.
\end{enumerate}
